# Supplementary material for: Unified theory for frequency combs in ring and Fabry-Perot quantum cascade lasers: an order-parameter equation approach
Source: arXiv:2403.06486 ancillary file (2024-03-11)
Supplement: Supplementary file 1 [file SupplementaryMaterial.pdf]

# Unified theory for frequency combs in ring and Fabry-Perot quantum cascade lasers: an order-parameter equation approach – Supplementary Material

Carlo Silvestri,[1] Massimo Brambilla,[2] Paolo Bardella,[3] and Lorenzo Luigi Columbo[3]

[1] *School of Electrical Engineering and Computer Science, The University of Queensland, Brisbane, QLD 4072, Australia*

[2] *Dipartimento Interateneo di Fisica, Politecnico di Bari and CNR-IFN, UOS Bari, Italy*

[3] *Dipartimento di Elettronica e Telecomunicazioni, Politecnico di Torino, 10129 Torino, Italy*

## I. DERIVATION OF THE SCALED EFFECTIVE SEMICONDUCTOR MAXWELL-BLOCH EQUATIONS

We want to show how the scaled effective semiconductor Maxwell-Bloch equations (ESMBEs) presented in Section II of the manuscript are obtained.

We start from the unscaled ESMBEs for the FP configuration [1]:

$$\frac{\partial E^+}{\partial z} + \frac{1}{v}\frac{\partial E^+}{\partial t} = -\frac{\alpha_{\rm L}}{2}E^+ + gP_0^+, \tag{S1}$$

$$-\frac{\partial E^-}{\partial z} + \frac{1}{v}\frac{\partial E^-}{\partial t} = -\frac{\alpha_{\rm L}}{2}E^- + gP_0^-, \tag{S2}$$

$$\frac{\partial P_0^+}{\partial t} = \frac{\Gamma(1+i\alpha)}{\tau_{\rm d}}\Big[-P_0^+ + if_0\varepsilon_0\varepsilon_{\rm b}(1+i\alpha)\big(N_0E^+ + N_1^+E^-\big)\Big], \tag{S3}$$

$$\frac{\partial P_0^-}{\partial t} = \frac{\Gamma(1+i\alpha)}{\tau_{\rm d}}\Big[-P_0^- + if_0\varepsilon_0\varepsilon_{\rm b}(1+i\alpha)\big(N_0E^- + N_1^-E^+\big)\Big], \tag{S4}$$

$$\frac{\partial N_0}{\partial t} = \frac{I}{eV} - \frac{N_0}{\tau_{\rm e}} + \frac{i}{4\hbar}\Big[E^{+*}P_0^+ + E^{-*}P_0^- - E^+P_0^{+*} - E^-P_0^{-*}\Big], \tag{S5}$$

$$\frac{\partial N_1^+}{\partial t} = -\frac{N_1^+}{\tau_{\rm e}} + \frac{i}{4\hbar}\Big[E^{-*}P_0^+ - E^+P_0^{-*}\Big]. \tag{S6}$$

where $E^+(z,t)$, $E^-(z,t)$ are the forward and backward envelopes of the electric fields, $P_0^+$, $P_0^-$ are the forward and backward polarization terms, $N_0$ is the zero-order density of carriers, and $N_1^+$, $N_1^-$ are the variable associated carrier grating due to SHB; $v$ is the group velocity, $\alpha_{\rm L}$ is the loss term, $\alpha$ is the LEF, $\tau_{\rm d}$ is the polarization dephasing time, $\Gamma$ is an adimensional costant proportional to the gain linewidth (see [2]), $f_0$ is the differential gain, $\varepsilon_0$ is the dielectric the vacuum dielectric constant, $\varepsilon_{\rm b}$ is the relative dielectric constant of the QCL medium, $I$ is the bias current, $V$ is the volume of the active region, $\tau_{\rm e}$ is the carrier lifetime, and the coefficient $g$ is given by:

$$g = \frac{-i\omega_0 N_{\rm p}\Gamma_{\rm c}}{2\varepsilon_0 n_{\rm r} c}, \tag{S7}$$

where $N_{\rm p}$ is the number of stages of structure, $\omega_0$ is the cold cavity angular frequency coinciding with the peak of the gain (used here as a reference frequency), $\Gamma_{\rm c}$ is the optical confinement factor in the active region, $c$ is the speed of light in the vacuum, and $n_{\rm r}$ is the effective background refractive index of the QCL medium. The ESMBEs are completed with the boundary conditions for the FP cavity:

$$E^-(L,t) = \sqrt{R}E^+(L,t), \tag{S8}$$

$$E^+(0,t) = \sqrt{R}E^-(0,t), \tag{S9}$$

where $L$ is the cavity length and $R$ is the reflectivity of QCL facets.
We aim to obtain the reduced model for the FP configuration, starting from Eqs. (S1)-(S6), under the assumption of fast carrier dynamics, which is well-suited for the case of QCL [3, 4], and near-threshold operation. Firstly we rewrite Eqs. (S1)-(S6) in dimensionless form. For this purpose, we introduce the following dimensionless dynamical

variables:

$$F^{+}=\sqrt{\frac{V\tau_e f_0'\epsilon_0\epsilon_b}{4\hbar}}E^{+}, \tag{S10}$$
$$F^{-}=\sqrt{\frac{V\tau_e f_0'\epsilon_0\epsilon_b}{4\hbar}}E^{-}, \tag{S11}$$
$$p^{+}=iA\sqrt{\frac{V\tau_e f_0'\epsilon_0\epsilon_b}{4\hbar}}P_0^{+}, \tag{S12}$$
$$p^{-}=iA\sqrt{\frac{V\tau_e f_0'\epsilon_0\epsilon_b}{4\hbar}}P_0^{-}, \tag{S13}$$
$$D_0=Af_0\epsilon_0\epsilon_b N_0, \tag{S14}$$
$$D_1^{+}=Af_0\epsilon_0\epsilon_b N_1^{+} \tag{S15}$$

where $A=\frac{v\tau_{\rm p}\omega_0 N_{\rm P}\Gamma_{\rm C}}{2\epsilon_0 n_{\rm r}c}$, $f_0'=\frac{f_0}{V}$, and $\tau_{\rm p}=(v\alpha_{\rm L}/2)^{-1}$. Then, we introduce dimensionless space and time variables, respectively $\eta$ and $t'$, expressed by:

$$\eta=\frac{z}{v\tau_d}, \tag{S16}$$
$$t'=\frac{t}{\tau_d} \tag{S17}$$

and we define the following parameters:

$$\sigma=\frac{\tau_d}{\tau_p} \tag{S18}$$
$$b=\frac{\tau_d}{\tau_e}, \tag{S19}$$
$$\mu=f_0'\epsilon_0\epsilon_b\frac{I\tau_{\rm e}}{e} \tag{S20}$$

Then, by using the quantities just defined, we can rewrite Eqs. (S1)-(S6) in the following form:

$$\frac{\partial F^{+}}{\partial\eta}+\frac{\partial F^{+}}{\partial t'}=\sigma\left[-F^{+}-p^{+}\right] \tag{S21}$$
$$-\frac{\partial F^{-}}{\partial\eta}+\frac{\partial F^{-}}{\partial t'}=\sigma\left[-F^{-}-p^{-}\right] \tag{S22}$$
$$\frac{\partial p^{+}}{\partial t'}=\Gamma(1+i\alpha)[-p^{+}-(1+i\alpha)\left(D_0F^{+}+D_1^{+}F^{-}\right)] \tag{S23}$$
$$\frac{\partial p^{-}}{\partial t'}=\Gamma(1+i\alpha)[-p^{-}-(1+i\alpha)\left(D_0F^{-}+D_1^{-}F^{+}\right)] \tag{S24}$$
$$\frac{\partial D_0}{\partial t'}=b\left[\mu-D_0+F^{+*}p^{+}+F^{-*}p^{-}+F^{+}p^{+*}+F^{-}p^{-*}\right] \tag{S25}$$
$$\frac{\partial D_1^{+}}{\partial t'}=b\left[-D_1^{+}+F^{-*}p^{-}+F^{+}p^{-*}\right] \tag{S26}$$

The boundary conditions are:

$$F^{-}(L',t')=\sqrt{R}F^{+}(L',t'), \tag{S27}$$
$$F^{+}(0,t')=\sqrt{R}F^{-}(0,t'), \tag{S28}$$

where $L'=\frac{L}{v\tau_d}$. We observe that the scaled polarization term $p^{+}$ in Eq. (S21) is preceded by a negative sign, thus functioning as a sink rather than a source. However, this is solely attributed to the introduction of scaling. Upon inspecting Eq. (S1), we notice how the unscaled forward polarization term acts as a source in the field equation. Hence, we comprehend that there is no error in the physical assumptions of the initial equations, and the aforementioned sign alteration arises from the chosen scaling approach. The same reasoning applies to the sign of $p^{-}$ in Eq. (S22).

## II. COMPARISON BETWEEN THE SINGLE SPATIOTEMPORAL EQUATION AND THE COUPLED CGLES

We numerically verify the equivalence between the single spatiotemporal equation, Eq. (40) in the main manuscript, and the two coupled CGLEs Eqs. (27)-(28), by integrating both models with identical parameters. For the single spatiotemporal equation, we solve it to obtain the dynamics of the auxiliary field $\psi$, and then reconstruct the forward and backward fields $F^+$ and $F^-$ following the procedure described in section III A of the main manuscript. As a specific example, we consider the case $K = 1$ (FP cavity) with the following parameters: $\alpha = 1.15$, $\tau_d = 0.1$ ps, $\Gamma = 0.06$, $p = 1.8$, $\sigma = 4.5 \times 10^{-4}$, and cavity length $L = 2$ mm. In Fig. S1, the temporal evolution of the power at $z = L$ (top panel) and the optical spectrum (bottom panel) for the same comb regime reproduced using the two approaches is illustrated. We observe perfect agreement between the results, thereby confirming the equivalence of the two approaches.

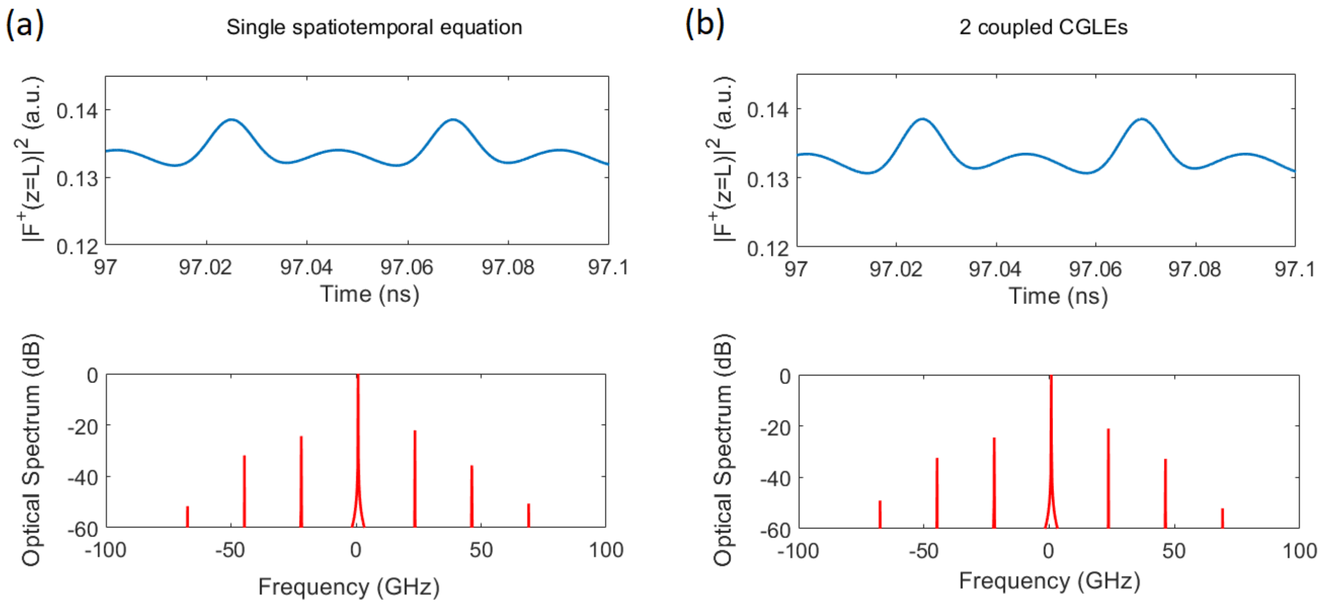


FIG. S1. Temporal evolution of the normalized power at the QCL facet (top) and optical spectrum (bottom) for a fundamental comb regime reproduced by integrating (a) the single spatiotemporal equation Eq. (40) in the main manuscript, and (b) the two coupled Complex Ginzburg-Landau Equations (CGLEs) Eqs. (27)-(28) in the main manuscript, by exploiting the same parameter set.

[1] C. Silvestri, L. L. Columbo, M. Brambilla, and M. Gioannini, Coherent multi-mode dynamics in a quantum cascade laser: amplitude- and frequency-modulated optical frequency combs, Opt. Express **28**, 23846 (2020).
[2] L. L. Columbo, S. Barbieri, C. Sirtori, and M. Brambilla, Dynamics of a broad-band quantum cascade laser: from chaos to coherent dynamics and mode-locking, Opt. Express **26**, 2829 (2018).
[3] J. Faist, F. Capasso, D. L. Sivco, C. Sirtori, A. L. Hutchinson, and A. Y. Cho, Quantum cascade laser, Science **264**, 553 (1994).
[4] J. Faist, G. Villares, G. Scalari, M. Rösch, C. Bonzon, A. Hugi, and M. Beck, Quantum cascade laser frequency combs, Nanophotonics **5**, 272 (2016).
